# Supplementary material for: "Good Robot!": Efficient Reinforcement Learning for Multi-Step Visual Tasks with Sim to Real Transfer
Source: arXiv:1909.11730 source file (2020-08-15)
Supplement: Supplementary file 2 [file 10appendix.tex]

% NOTE: A bunch of the appendix figures and notes are outdated as of June 2020

The appendix contains several additional figures and metrics. 
These include the percentage of successful grasps, placement action efficiency, and trial completion rate.
The completion rate is defined as the percentage of trials where the policy is able to successfully complete a task before the grasp or push action fails 10 consecutive times.
Success of a push is when more than 300 depth pixels have changed in a scene. 
A successful grasp is counted upon two consecutive detections by the internal Robotiq grasp sensor, once upon closing and once after lifting.
A successful place for stacking is evaluated more specifically by the maximum $z$ height in the heightmap. 
Alternately it can be awarded when height the highest vertical $z$ height of a scene has increased by a minimum threshold.

\subsection{Extended experiment notes}
\textbf{Clear 10 Toys, Simulation:} We establish a baseline via the primary simulated experiment found in VPG~\cite{zeng2018vpg}, where 10 toys with varied shapes must be grasped to clear the robot workspace.
Some differences occur because we also account for our asymmetric gripper, which means training cannot automatically be applied at the both the actual gripper rotation angle and its 180\degree offset. Fig.~\ref{fig:gripper_asymmetry_time_dependencies} shows such considerations in detail.
Additionally, our training performs experience replay in parallel with robot actions. 
The SPOT Framework matches VPG\cite{zeng2018vpg} with 100\% task completion, and improves both grasp successes from 68\% to 84\% and action efficiency from 64\% to 74\%.
% EVT reduces the Action Efficiency Error (1 - Action Efficiency) from 39\% with VPG to 14\% with EVT. % formerly 18.3\%

Table~\ref{table:PushingGraspingResults} (top) shows the results. As this is a fairly straightforward task, all methods are eventually able to complete it in the basic case, but we see that SPOT-Q training leads to the highest grasp success rate, but there is not a dramatic difference.
% This makes intuitive sense, since the task structure is very simple.

\textbf{Clear Toys Adversarial:} The second baseline scenario is 11 challenging adversarial arrangements from VPG~\cite{zeng2018vpg} where toys are placed in tightly packed configurations. 
We use the pretrained weights from the ``Clear 10 Toys'' task in scenarios the algorithm has never previously seen.
% The evaluation algorithm defined by VPG~\cite{zeng2018vpg} is designed such that when no successful grasp is made for 10 consecutive actions the task is considered incomplete.
We validate on 10 trials for each of the 11 challenging arrangements, and our model was able to clear the scene in 104 out of 110 trials. 
Table~\ref{table:PushingGraspingResults} (bottom) details the results.
% : SPOT-Q performed substantially better.
% In EVT's lone failure case the model had successfully separated the tightly packed blocks on the final 10th action without a successful grasp.
% It is reasonable to expect it would have finished clearing the scene in the next few actions had it not hit the incomplete task limit.

Curiously, while the rate of tasks completed rises, action efficiency is reduced in these challenging arrangements.
Subjectively, this is due to the higher priority placed on grasping when compared to pushing as the SPOT-Q model attempts pushes in 10\% of actions in these scenarios on average. 
In many cases the algorithm attempts a push only after several failed attempts at grasping, which finally frees up the blocks to complete the task, while in other cases it separates blocks using grasps alone.

\section{Technical design notes}

We expect that with minor optimizations in our code, a real robot could easily take an action once every 8 seconds.
In future work a less simplistic action sequence could ensure that
the robot moves completely out of the frame only as needed,
allowing it to act many times faster.

\subsection{Real Robot}

Real robot training for block stacking takes approximately 12 hours at 20 seconds per action.
We run simulated training for sim to real transfer of stacks and rows over 20k actions, also in real time at 15 seconds per action which takes approximately 3.5 days.
% At test time the real robot runs at a rate of 15 seconds per action, and the difference is accounted for by experience replay running in a parallel Python thread.
Unstacking during real world training and testing is largely automated by retaining a queue of past place locations which are grasped and randomly released in reverse order after a trial is complete.
We periodically return objects which have left the robot workspace by hand, but a physical barrier like our bin in~\cite{hundt2019costar} would suffice. 
The bin was excluded for consistency with the VPG~\cite{zeng2018vpg} baseline.

\subsection{Grid world progress reward implementation}

Progress reward is adapted to the Grid World environment by first applying the wavefront expansion algorithm to assign distance to goal (excluding turns) at each grid position. This BFS distance is then inverted, and sum-normalized to derive the instantaneous reward function. In addition to returning this instantaneous reward at each timestep, situation removal is implemented by triggering a hard environment reset with 0 reward in instances of progress reversal (decrease in reward or more than 2 consecutive turns).
\begin{table*}\centering
\vspace{0.2cm}
% \ra{1.3}
\begin{tabular}{LLLLCCCCCCRRRR@{}}\toprule
\rowcolor{white} \textbf{Simulation} & Source & Algorithm Ablation & Action & Scenarios & Trials & Grasp & Action\\
\midrule
% Clear 10 Toys & VPG\cite{zeng2018vpg} &Baseline (eq. \ref{eq:vpg})&Standard& 94\% (100\%)& 94\% (100\%) & 79\% (68\%) & 68\% (61\%)\\ %
Clear 10 Toys & VPG~\cite{zeng2018vpg} &Baseline (eq. \ref{eq:vpg})&Standard&100\%& 100\% & 68\% & 61\%\\ % 2020-02-16-21-33-55_Sim-Push-and-Grasp-Two-Step-Reward-Training
% Clear 10 Toys & *VPG\cite{zeng2018vpg} &Baseline (eq. \ref{eq:vpg})&Standard& 94\%& 94\% & 83\% & 61\%\\
% \rowcolor{white}Clear 10 Toys& Ours &Baseline (eq. \ref{eq:vpg})&Standard& 100\%& 100\% & 87\% & 82\%\\ % 2019-09 EVT Efficientnet Run
% Clear 10 Toys & Ours &SPOT (eq. \ref{eq:spott})&Standard& 100\%& 100\% & \textbf{87\%} & \textbf{86\%}\\ % 2019-09 EVT Efficientnet run
\rowcolor{white}Clear 10 Toys & Ours &SPOT (eq. \ref{eq:spott})&Standard& 100\%& 100\% & \textbf{83\%} & \textbf{73\%}\\ % 2020-02-16-21-37-47_Sim-Push-and-Grasp-SPOT-Trial-Reward-Training\rowcolor{white}
Clear 10 Toys & Ours &SPOT-Q (eq. \ref{eq:spott} and \ref{eq:spot_q})& Masked & 100\%& 100\% & \textbf{84\%} & \textbf{74\%}\\ % 
\midrule
% \rowcolor{white}Clear Toys Adversarial& VPG~\cite{zeng2018vpg} &Baseline (eq. \ref{eq:vpg})&Standard& 5/11 (5/11) & 94\% (84\%) & 42\% (77\%) & 42\% (60\%)\\
\rowcolor{white}Clear Toys Adversarial& VPG~\cite{zeng2018vpg} &Baseline (eq. \ref{eq:vpg})&Standard& 5/11 & 84\% & 77\% & 60\%\\
% \rowcolor{white}Clear Toys Adversarial& Ours&Baseline (eq. \ref{eq:vpg})&Standard& \textbf{10/11} & \textbf{99\%} & 62\% & 51\%\\ % 2019-09 EVT EfficientNet Run
Clear Toys Adversarial& Ours&SPOT (eq. \ref{eq:spott})&Standard& \textbf{6/11} & \textbf{94\%} & 37\% & 36\%\\ % 2020-02-16-21-37-47_Sim-Push-and-Grasp-SPOT-Trial-Reward-Training
\rowcolor{white}Clear Toys Adversarial& Ours&SPOT-Q (eq. \ref{eq:spott} and  \ref{eq:spot_q})&Masked& \textbf{7/11} & \textbf{95\%} & 46\% & 38\%\\ % 2020-02-16-21-33-59_Sim-Push-and-Grasp-SPOT-Trial-Reward-Common-Sense-Training, results inside that folder: 2020-02-19-22-05-10_Sim-Push-and-Grasp-SPOT-Trial-Reward-Common-Sense-Challenging-Arrangements
\bottomrule
\end{tabular}
\caption{\label{table:AppendixPushingGraspingResults}  Pushing and grasping baseline simulation results. The first task is to clear 10 toys for 100 trials with random arrangements, and the second is to clear 10 trials each across 11 adversarial arrangements with 110 total trials. Bold entries highlight our key algorithm improvements over the baseline. 
We train for 5k total actions with an allowance permitting the final trial to complete. 
``Trials Complete'' indicates all objects are cleared. 
``Grasp'' indicates the average percentage of successful grasp attempts.}
\vspace{-0.2cm}
\end{table*}

\begin{table*}\centering
% \ra{1.3}
\begin{tabular}{LLLCCCCCCCRRRR@{}}\toprule
\rowcolor{white}\textbf{Simulation} & Algorithm &Action& Trials & Grasp & Place & Action\\
\rowcolor{white}Test Task& Ablation &Space& Complete & & & Efficiency\\
\midrule
Stack of 4 Cubes& Baseline (eq. \ref{eq:vpg}) &Standard& 13\% & 94\% & 58\% & 2\%\\ % costar 2020-04-25-21-41-04_Sim-Stack-Two-Step-Reward-Training/2020-04-27-17-44-27_Sim-Stack-Two-Step-Reward-Testing/best_stats.json
% Stack of 4 Cubes& Baseline (eq. \ref{eq:vpg}) &Standard& 5\% & 84\% & 45\% & 4\%\\ % Note this is an EVT EfficientNet based Model from sep 2019
Stack of 4 Cubes& Baseline (eq. \ref{eq:vpg})  $\times TP_t/TP_{max}$  &Standard& 57\% & 29\% & 63\% & 29\%\\ % 2020-02-21-20-33-47_Sim-Stack-Two-Step-Reward-Training
% \rowcolor{white}Stack of 4 Cubes& SPOT (eq. \ref{eq:situationremoval}) &Standard& 74\% & 93\% & 83\% & 63\%\\ % Note this is an EVT EfficientNet run from sep 2019

\rowcolor{white}Stack of 4 Cubes & SPOT (eq. \ref{eq:spott}) &Masked& 91\% & 73\% & 64\% & 31\%\\ % 2020-02-20-16-20-23_Sim-Stack-SPOT-Trial-Reward-Common-Sense-Training
Stack of 4 Cubes & SPOT (eq. \ref{eq:spott}) & Standard & 97\% & 81\% & 79\% & 38\%\\
\rowcolor{white}Stack of 4 Cubes& SPOT-Q (eq. \ref{eq:spott} and \ref{eq:spot_q}) &Masked& \textbf{98\%} & \textbf{81\%} & \textbf{84\%} & \textbf{57\%}\\ % 2020-02-16-22-38-38_Sim-Stack-SPOT-Trial-Reward-Testing DenseNet, on CoSTAR, loose action boundaries
% \rowcolor{white}\textbf{Real}&Stack of 4 Cubes& SPOT (eq. \ref{eq:spott}) &Masked (eq. \ref{eq:spot_q})& \textbf{82\%} & \textbf{71\%} & \textbf{82\%} & \textbf{60\%}\\ % 2020-02-09-11-02-57_Real-Stack-SPOT-Trial-Reward-Common-Sense-Training
\midrule

\rowcolor{white}Row of 4 & Baseline (eq. \ref{eq:vpg}) &Standard& 13\% & 59\% & 25\% & 1\%\\ % costar 2020-04-25-21-41-35_Sim-Rows-Two-Step-Reward-Training/2020-04-27-17-25-31_Sim-Rows-Two-Step-Reward-Testing/best_stats.json
% Rows Trial Data: https://github.com/jhu-lcsr/costar_visual_stacking/releases/tag/v0.12.0
Row of 4 & SPOT (eq. \ref{eq:spott}) &Standard& 92\% & 68\% & 61\% & 29\%\\ % NOTE THIS IS THE EFFICIENTNET MODEL FROM 2019-09, action efficiency is 44% assuming ideal 6 actions per row, 29% for 4 actions per row
\rowcolor{white}Row of 4 & SPOT-Q &Masked& \textbf{93\%} & \textbf{87\%} & \textbf{85\%} & \textbf{57\%}\\ % NOTE THIS IS THE DENSENET MODEL FROM 2020-02-10-18-38-48_Sim-Rows-SPOT-Trial-Reward-Common-Sense-Training action efficiency is 86% assuming ideal 6 actions per row, 57% assuming ideal 4 actions per row.

% \midrule
% \rowcolor{white}Stack Toys 0.2m &  SPOT (eq. \ref{eq:spott}) &Masked (eq. \ref{eq:spot_q})& 24\%& 55\% & 48\% & 4\%\\ % 2020-02-10-19-09-09_Sim-Stack-SPOT-Trial-Reward-Common-Sense-Training
% \midrule
\bottomrule
\end{tabular}
\caption{\label{table:AppendixStackingResults} Multi-Step task test success rates measured out of 100\% for simulated tasks involving push, grasp and place actions trained for 10k actions.
Bold entries highlight our key algorithm improvements over the baseline.}
\vspace{-0.2cm}
\end{table*}

\begin{table*}\centering
% \ra{1.3}
\begin{tabular}{LLLLCCCCCCRRRR@{}}\toprule
\rowcolor{white}\textbf{Real} & Training & Algorithm & Action & Trials & Grasp & Place & Action & Training\\
\rowcolor{white}Test Task & Domain & & Space & Complete & & & Efficiency& Actions\\
\midrule
% \rowcolor{white}Clear 10 Toys & VPG~\cite{zeng2018vpg} &Baseline (eq. \ref{eq:vpg})&Standard& TODO\% & TODO\% & TODO\% & TODO\% \\
Clear 20 Toys & Real & SPOT-Q (eq. \ref{eq:spot_q})&Masked& 1/1& 75\% & -  & 75\%&1k\\
\midrule
\rowcolor{white}Stack of 4 Cubes & Real & SPOT-Q (eq. \ref{eq:spott} and \ref{eq:spot_q}) &Masked& 82\% & 71\% & 82\% & 60\% &2.5k\\ % 2020-02-09-11-02-57_Real-Stack-SPOT-Trial-Reward-Common-Sense-Training
Stack of 4 Cubes & Sim & SPOT-Q (eq. \ref{eq:spott} and \ref{eq:spot_q}) &Masked& \textbf{90\%} & 80\% & 80\% & 59\%&10k\\ % 2020-02-22-17-52-17_Real-Stack-SPOT-Trial-Reward-Common-Sense-Testing

\midrule
\rowcolor{white}Row of 4 Cubes & Sim &SPOT-Q (eq. \ref{eq:spott} and \ref{eq:spot_q})&Masked& \textbf{80\%}& 68\% & 89\% & 71\%&10k\\
% Our action efficency was 107 at 6 actions per row, which is 71\% assuming it takes 4 actions per row 1.07*(4/6).
\bottomrule
\end{tabular}
\caption{\label{table:AppendixRealResults}Real robot task results. Bold entries highlight sim to real transfer.}
\vspace{-0.5cm}
\end{table*}

\begin{figure}[b!]
    % \centering
    % \hfill
    % \includegraphics[width=\columnwidth]{grasp_efficiency.pdf}
    % \includegraphics[width=\columnwidth]{2019-09-12-18-21-37-push-grasp-16k-trial-reward_success_plot}
    % \includegraphics[width=\columnwidth]{2020-02-10-18-38-48_Sim-Rows-SPOT-Trial-Reward-Common-Sense-Training-Sim-Rows-SPOT-Trial-Reward-Common-Sense-Training_success_plot.png}
    \includegraphics[width=\columnwidth]{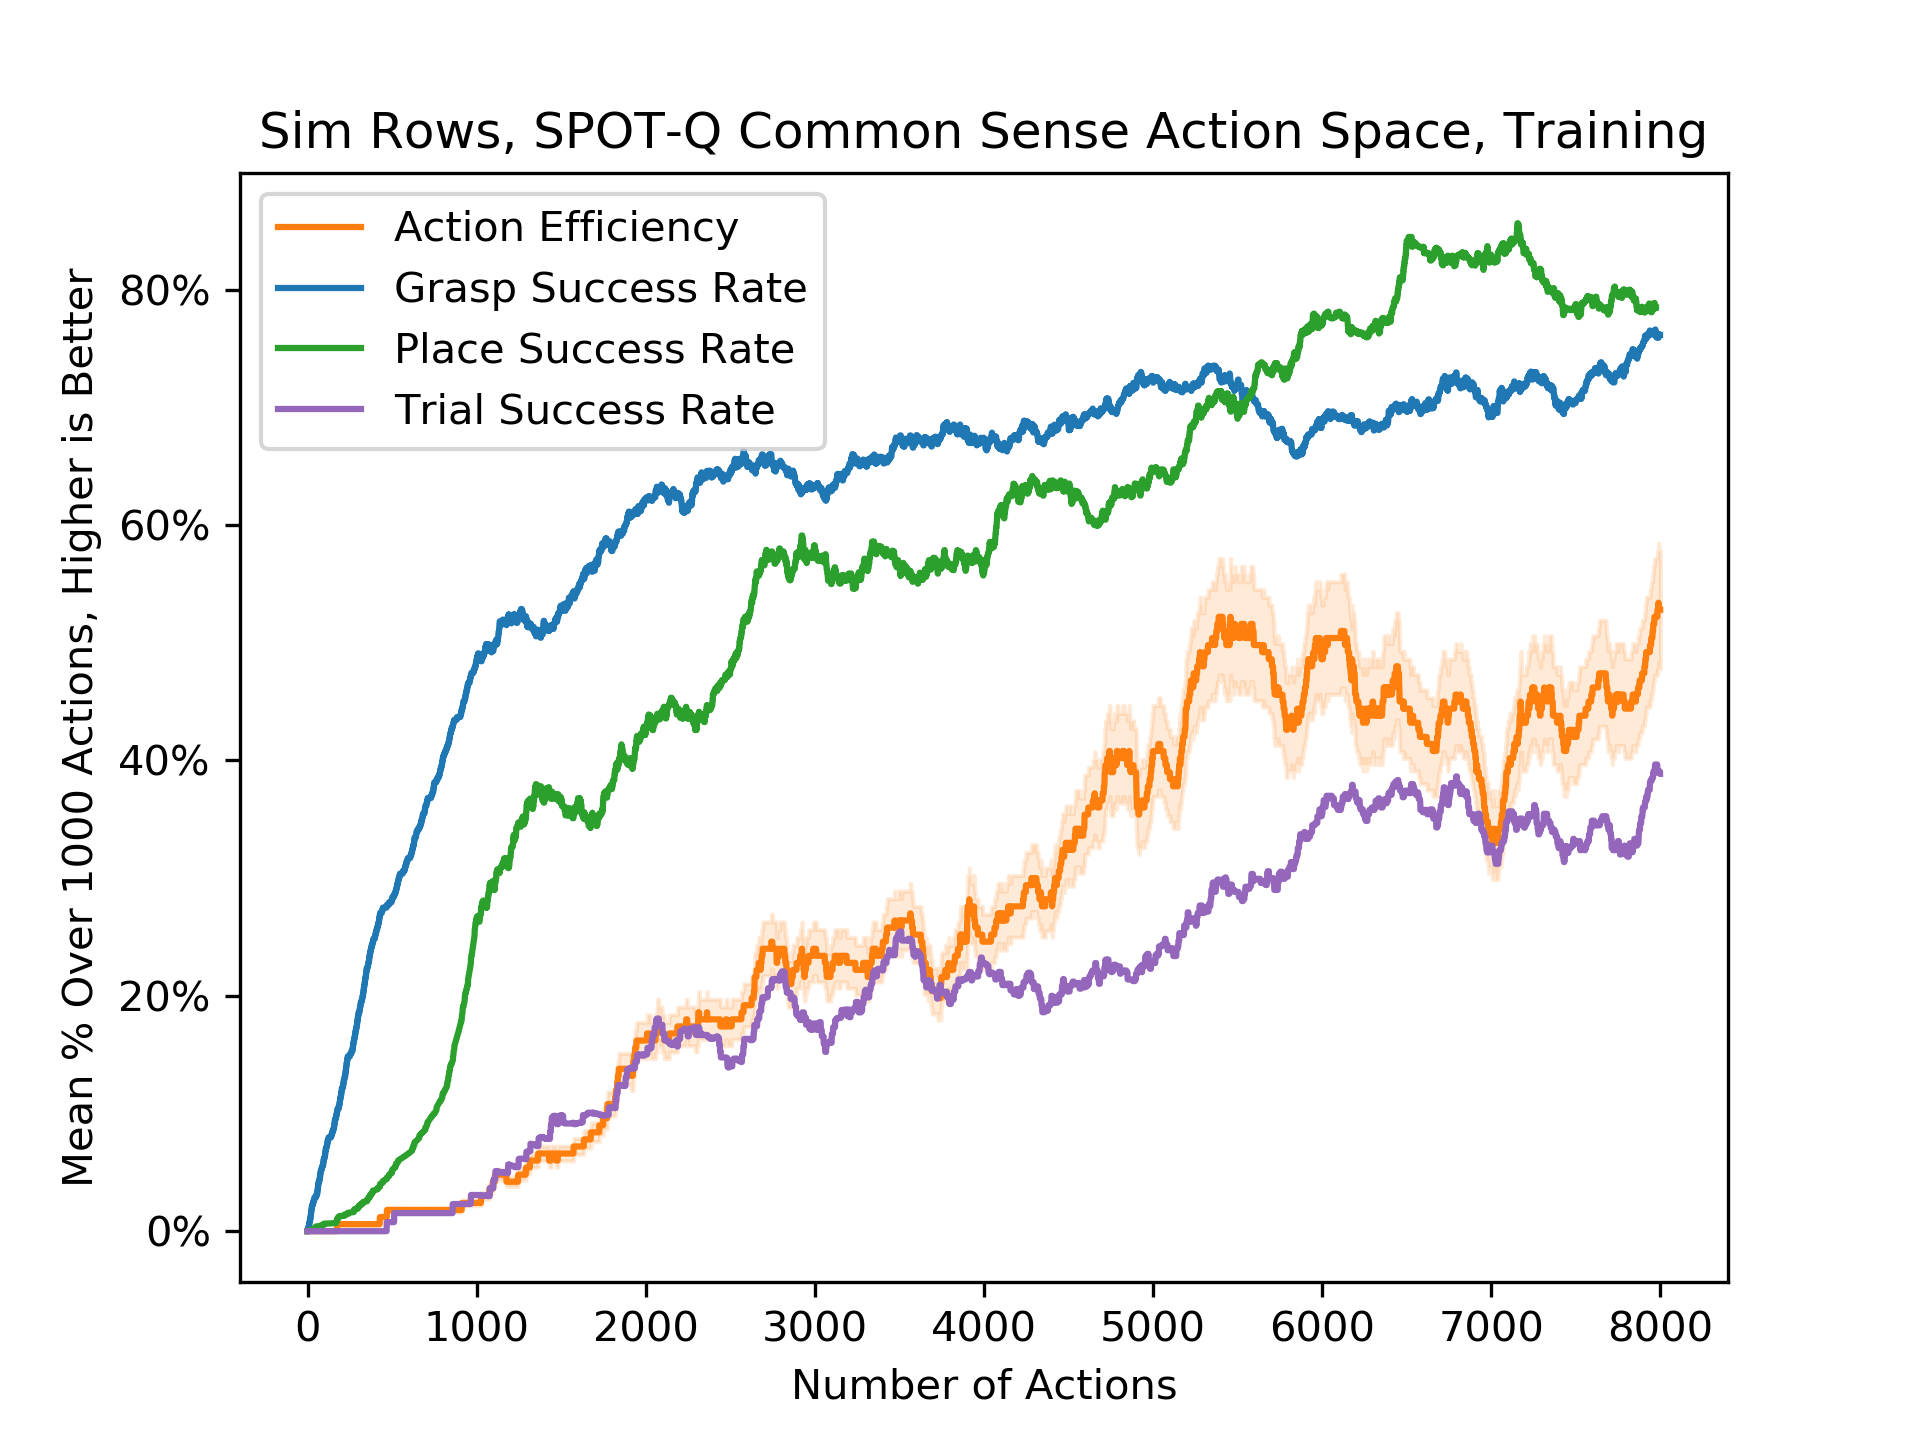}
    \caption{
    \label{fig:grasp_efficiency}
    Grasp Success Rate, Trial Success Rate, and Action Efficiency improvement during simulated SPOT Rows Training. Higher is better.
    Notice the final 40\% training trial success rate is much lower than the test rate of 93\%. 
    This is because situation removal is applied and the scene is reset during training when an action decreases the current row length, but is not a part of the final model testing.
}
\vspace{-0.5cm}
\end{figure}

\begin{figure}[bt!]
    % \centering
    % \hfill
    % \includegraphics[width=\columnwidth]{grasp_place_stack_efficiency}
    % \includegraphics[width=\columnwidth]{2020-02-09-11-02-57_Real-Stack-SPOT-Trial-Reward-Common-Sense-Training-Real-Stack-SPOT-Trial-Reward-Common-Sense-Training_success_plot.png}
    \includegraphics[width=\columnwidth]{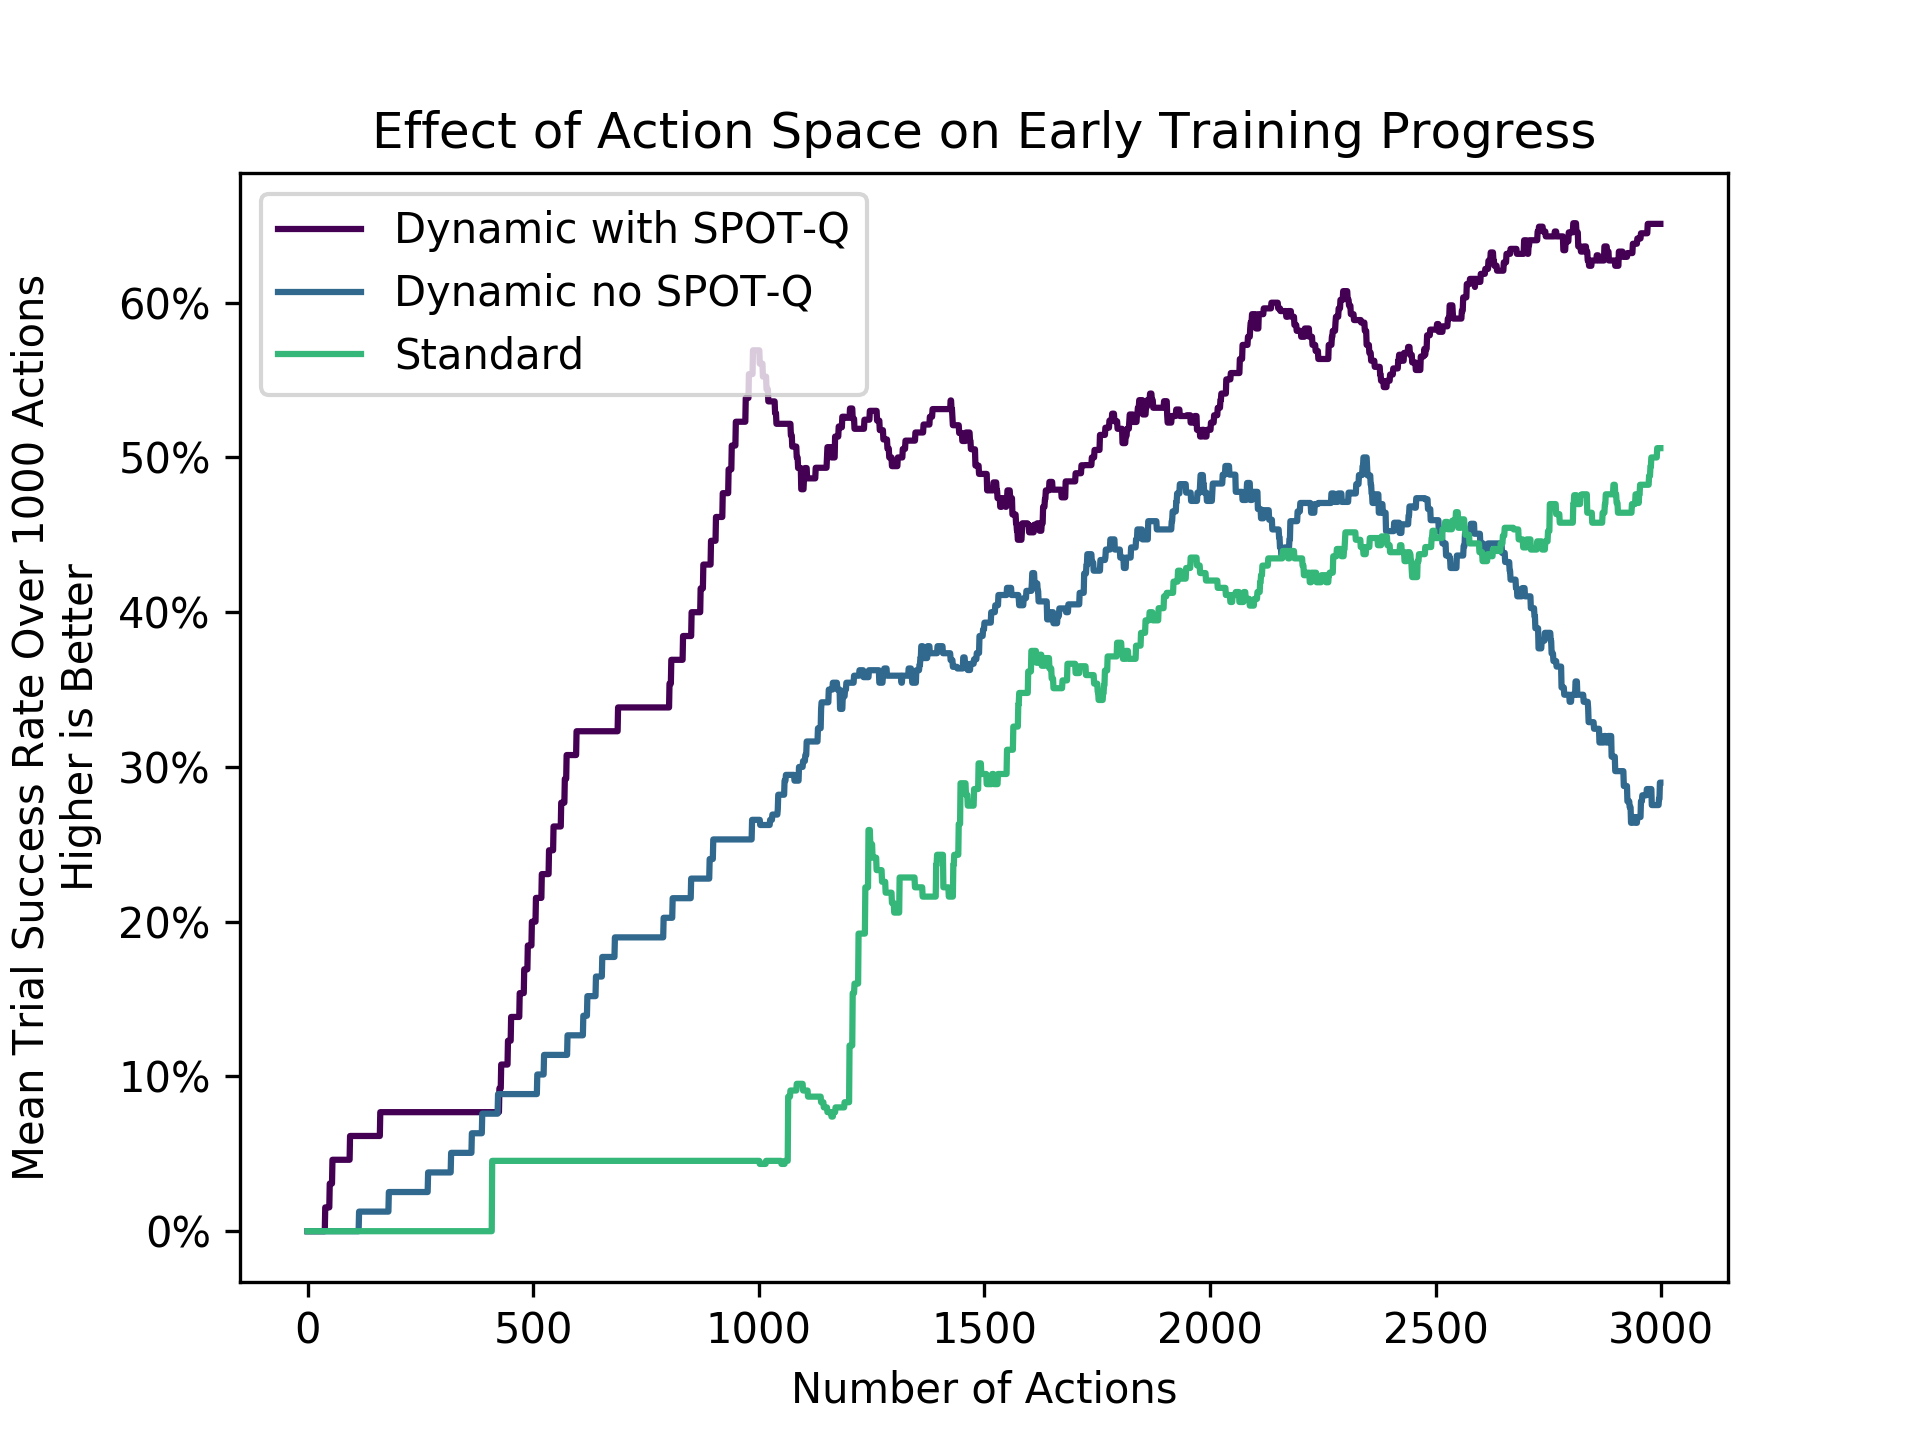}
    \caption{
    \label{fig:spot-q-early-training-progress}
    The advantage of a masked action space with SPOT-Q is clear in this comparison of early simulated stacking progress.
}
% \vspace{-0.5cm}
\end{figure}

\begin{algorithm*}[bt!]
\caption{SPOT-Q with Prioritized Experience Replay}
\label{alg:spot_q_replay_extended}
\begin{algorithmic}
\State \textbf{Input} Replay Memory $H_T=(S_T, A_T, \text{trial reward } R_T, \text{instant reward } \Gamma_T, \text{prediction } P_T, \text{action type } \Phi_T, \text{budget } B)$
\For {b in B}
    \While {$\Call{agent\_taking\_action\_in\_parallel}{\pi(s_b))}$}
        % \LineComment{, ensuring the action type matches $\Phi_{b-1}$ but success does not.}
        \State $I = \argsort(\, \abs{R_T-P_T} )\text{ then with }P(0.95)\text{ filter }I\text{ s.t. } \Phi_t = \Phi_{b-1} \text{ and } \Call{success}{H_{t}} \not= \Call{success}{H_{b-1}}$
        \State $t \sim P(t) = \Call{power}{ I; 2}$ \Comment{Sample $t$ from power distribution of indices $I$ sorted in surprise order.}
        % \State $t \sim P(t) = \Call{power}{\argsort(\, \abs{R_T-P_T} ) ; 2}$ \Comment{Sample $t$ from power distribution in surprise order.}
        % \LineComment SPOT-Q $y_{M,t} =$ eq. \ref{eq:spot_q} creates a second label $R_{\pi(s_{t})}\!=\!0$ if $\pi(s_{t})\not\in M(S_t, A_t)$ where $M\!=\!$ eq. \ref{eq:dynamic-action-space}.
        \LineComment{SPOT-Q $y_{M,t}\!=$ eq. \ref{eq:spot_q} adds label 0 if $\pi(s_{t})\not\in M(S_t, A_t)$}
        \State $\delta_{R,t} = \Call{huber\_loss}{Q(s_t,a_t) ;\; y_{M,t}(R_T; S_T; A_T)}$ \Comment SPOT-Q, trial reward $R_{trial} =$ eq. \ref{eq:spott}
        \State $\Call{backprop}{\sum{}{\delta_{R,t}}}$; step optimizer; weights update. 
        \LineComment{Unlike PER\cite{schaul2016prioritized}, we do not update P here because $B \leq 20$k is too small.}
    \EndWhile
    \State{\Call{update}{$H_T$}} \Comment{The action and/or trial is complete. Add in most recent sample $H_b$ and update $R_T$ if possible.}
    \State $\delta_{\Gamma,b-1} = \Call{huber\_loss}{Q(s_{b-1},a_{b-1}) ;\; y_{M,b-1}(\Gamma_{b-1}; S_T; A_T)}$ \Comment{SPOT-Q, instant reward $\Gamma_{\spot} =$ eq. \ref{eq:spot} }
    \State $\Call{backprop}{\sum{}{\delta_{\Gamma,b-1}}}$; step optimizer; weights update.
\EndFor
\end{algorithmic}
\end{algorithm*}

\begin{table}\centering
\vspace{0.2cm}
% \ra{1.3}
\begin{tabular}{LLCCCCCCCCRRRR@{}}\toprule
\rowcolor{white} \textbf{Simulation} & Algorithm & Mask & Cases & Trials & Efficiency\\
% \rowcolor{white}Test Task& Ablation &Space& 100\% Complete &Complete& Efficiency\\
\midrule
% Clear 10 Toys & VPG\cite{zeng2018vpg} &Baseline (eq. \ref{eq:vpg})&\xmark& 94\% (100\%)& 94\% (100\%) & 79\% (68\%) & 68\% (61\%)\\ %
Clear Toys & VPG~\cite{zeng2018vpg} &\xmark&100\%& 100\% & 61\%\\ % 2020-02-16-21-33-55_Sim-Push-and-Grasp-Two-Step-Reward-Training
% Clear 10 Toys & *VPG\cite{zeng2018vpg} &Baseline (eq. \ref{eq:vpg})&\xmark& 94\%& 94\% & 83\% & 61\%\\
% \rowcolor{white}Clear 10 Toys& Ours &Baseline (eq. \ref{eq:vpg})&\xmark& 100\%& 100\% & 87\% & 82\%\\ % 2019-09 EVT Efficientnet Run
% Clear 10 Toys & Ours &SPOT (eq. \ref{eq:task_progress})&\xmark& 100\%& 100\% & \textbf{87\%} & \textbf{86\%}\\ % 2019-09 EVT Efficientnet run
\rowcolor{white}Clear Toys & $R_{\text{trial}}$ &\xmark& 100\%& 100\% & \textbf{73\%}\\ % 2020-02-16-21-37-47_Sim-Push-and-Grasp-SPOT-Trial-Reward-Training\rowcolor{white}
Clear Toys & SPOT F.W. & \cmark & 100\%& 100\% & \textbf{74\%}\\ % 
\midrule
% \rowcolor{white}Clear Toys Adversarial& VPG~\cite{zeng2018vpg} &Baseline (eq. \ref{eq:vpg})&\xmark& 5/11 (5/11) & 94\% (84\%) & 42\% (77\%) & 42\% (60\%)\\
\rowcolor{white}Adversarial& VPG~\cite{zeng2018vpg} & \xmark& 5/11 & 84\% & 60\%\\
% \rowcolor{white}Clear Toys Adversarial& Ours&Baseline (eq. \ref{eq:vpg})&\xmark& \textbf{10/11} & \textbf{99\%} & 62\% & 51\%\\ % 2019-09 EVT EfficientNet Run
Adversarial & $R_{\text{trial}}$ &\xmark& \textbf{6/11} & \textbf{94\%} & 36\%\\ % 2020-02-16-21-37-47_Sim-Push-and-Grasp-SPOT-Trial-Reward-Training
\rowcolor{white}Adversarial & SPOT F.W. &\cmark& \textbf{7/11} & \textbf{95\%} & 38\%\\ % 2020-02-16-21-33-59_Sim-Push-and-Grasp-SPOT-Trial-Reward-Common-Sense-Training, results inside that folder: 2020-02-19-22-05-10_Sim-Push-and-Grasp-SPOT-Trial-Reward-Common-Sense-Challenging-Arrangements
\bottomrule
\end{tabular}
\caption{\label{table:PushingGraspingResults}  Pushing and grasping baseline simulation results. The first task is to clear 10 toys for 100 trials with random arrangements, and the second is to clear 10 trials each across 11 adversarial arrangements with 110 total trials.
Bold entries highlight our key algorithm improvements over the baseline. 
We train for 5k total actions with an allowance permitting the final trial to complete. 
``Trials'' indicates the overall rate at which all objects are cleared.
``Cases'' indicates the number of specific adversarial arrangements which were cleared in all 10 trials with that arrangement.
All ``Clear Toys'' random arrangement cases were cleared successfully.
% ``Grasp'' indicates the average percentage of successful grasp attempts.
}
\vspace{-0.2cm}
\end{table}

\textbf{Stack 4 Cubes:} Our primary test task is to stack 4 cubes randomly placed within the scene. 
During training, we ensure that workspace constraints are strictly observed by deeming any action in which a partially assembled stack is subsequently toppled returns a reward of 0 and immediately ends the training trial with the failure condition. 
This strict progress evaluation criteria ensures the scores indicate an understanding of the context surrounding the stack.

In simulation we evaluate the baseline $R_{\text{base}}$ (eq.~\ref{eq:vpg}) reward; adding Situation Removal,  $R_{\progress}$ (eq.~\ref{eq:instant_progress}) with task progress and situation removal; and SPOT-Q (eq.~\ref{eq:spotq}), which dynamically restricts the action space and trains choices outside that action space with an assumed reward of 0.
Table~\ref{table:StackingResults} shows the results.
As evidenced by the huge difference between SPOT and the baseline reward schedule, the SPOT reward proves essential to task completion, succeeding 97\% of the time, versus only 57\% without it.
SPOT-Q, in turn, provides a slightly better 98\% completion rate with an even more important increase in action efficiency from 38\% to 57\%.

\textbf{Row of 4 Cubes:} Our third test task evaluates the ability of the algorithm to generalize across tasks.
Curiously, while making a row of 4 blocks appears similar to stacking, it is more difficult to train. 
In particular, whereas with stacking optimal placement occurs on top of a strong visual feature---another block---the arrangement of blocks in rows depends on non-local visual features, i.e.~the rest of the row.
Additionally, every block in each row is available for grasping, which may reverse progress, as opposed to stacks where only the top block is readily available.
This requires significant understanding of context, as we have described it, to accomplish.
Table~\ref{table:StackingResults} shows our algorithm's performance on this difficult task, succeeding 93\% of the time.

\begin{table}[h]
\caption{Notation}\smallskip
\centering
\resizebox{.95\columnwidth}{!}{
\smallskip\begin{tabular}{r l}
$\pi$ & the policy eq. \ref{eq:policy_pi} trained Neural Network \\
$s_t$ & the state at time $t$, the depth and rgb heightmap images \\
$a_t$ & the action at time $t$. $a \in A$ \\
$A$ & the set of all possible actions \\
$\pi(s_t) $ & the action the policy predicts from state $s_t$.\\
$y_t$ & the target value, eq. \ref{eq:q-learning} \\
$R(s_{t+1}, a_t)$ & the reward at time $t$. \\
$\gamma$ & Time discount factor. \\
$Q(s_t, a_t)$ & The quality function. \\
$\phi_t$ & The value of the sub task at a specific time. \\
$\Gamma(\phi_t)$ & Task indicator, a specific reward weight \\
$\Gamma_{SPOT}(\phi_t)$ & Instantaneous SPOT reward \\
% $\Gamma_{pos}$ & I'm not sure. (removed) \\
$TP_t$ & task progress at this time step aka action index \\
$TP_{max}$ & the maximum possible value for task progress \\
$N$ & The last time step in a trial. \\
$R_{trial}(s_{t+1}, a_t)$ & The SPOT trial reward at time T, the last time step in a trial. \\
$T$ & (1) The size of the replay buffer in Alg. \ref{alg:spot_q_replay}, equivalent \\
& to the total number of actions that have passed, or \\
& (2) the final time step of a single trial.  \\
$H_T$ & The replay memory. \\
$S_T$ & A set of states. $S_T = \{s_i\}_{i=1}^{T}$ \\
$A_T$ & A set of actions. $A_T = \{a_i\}_{i=1}^{T}$ \\
$R_T$ & A set of rewards. $R_T = \{r_i\}_{i=1}^{T}$ \\
$P_T$ & A set of predictions previously made by the\\
& network $\pi_t(s_t)$. $P_T = \{p_i\}_{i=1}^{T}$ \\
% $v_t$ & The target? Should this be $y_t$? \\
$a_{\pi, t}$ & The action the current policy \\ & \textbf{would have taken} given state $s_t$ \\
$\delta_t$ & the loss\\
$M_t(A)$ & A masking of desired actions at time $t$. \\ & $M_t(A) \subset A$. \\
$\pi_M$ & The best action allowed by the mask. \\
$\Phi$ & Set of all sub-tasks (action types), like push, grasp, place. \\
\end{tabular}
}
\label{notation}
\end{table}
